# Supplementary material for: Experimental Adiabatic Quantum Factorization under Ambient Conditions Based on a Solid-State Single Spin System
Source: arXiv:1611.03293 source file (2016-11-10)
Supplement: Supplementary file 1 [file Supplementary_Material.pdf]

# Supplementary Material for Experimental Adiabatic Quantum Factorization under Ambient Conditions Based on a Solid-State Single Spin System

Kebiao Xu,[1] Tianyu Xie,[1] Zhaokai Li,[1,2] Xiangkun Xu,[1] Mengqi Wang,[1] Xiangyu Ye,[1] Fei Kong,[1] Jianpei Geng,[1] Changkui Duan,[1] Fazhan Shi,[1,2] and Jiangfeng Du[1,2]

[1]*Key Laboratory of Microscale Magnetic Resonance and Department of Modern Physics, University of Science and Technology of China, Hefei 230026, China*

[2]*Synergetic Innovation Center of Quantum Information and Quantum Physics, University of Science and Technology of China, Hefei, 230026, China*

## THEORETICAL DESCRIPTION

### 1.1 Hamiltonian

The total Hamiltonian of system with the control pulse is

$$H = H_0 + H(t), \tag{S1}$$

$$H_0 = H_{\parallel} + H_{\perp}, \tag{S2}$$

$$H_{\parallel} = DS_z^2 + \gamma_e B_z S_z + QI_z^2 + \gamma_n B_z I_z + A_{\parallel} S_z I_z, \tag{S3}$$

$$H_{\perp} = A_{\perp}(S_x I_x + S_y I_y). \tag{S4}$$

$H_0$ is the Hamiltonian of the system consists of a negatively charged NV center and a adjacent $^{14}$N, as we have described in the main text. $H(t)$ is the Hamiltonian of applied microwave (MW) and radio-frequency (RF) pulses, detailed expressions are

$$H(t) = H_{MW}(t) + H_{RF}(t), \tag{S5}$$

$$H_{MW}(t) = \gamma_e B_1(t) Cos(\omega_1 t + \psi_1(t))(S_x + \frac{\gamma_n}{\gamma_e} I_x), \tag{S6}$$

$$H_{RF}(t) = \gamma_n B_2(t) Cos(\omega_2 t + \psi_2(t))(I_x + \frac{\gamma_e}{\gamma_n} S_x). \tag{S7}$$

As $\gamma_e = 2.802\ MHz/G$ and $\gamma_n = 0.30766\ kHz/G$, $\gamma_e$ is three orders of magnitude larger than $\gamma_n$, in Eq. S6 the $I_x$ term can be ignored, but the $S_x$ term in Eq. S7 can not. We carried out the experiment in the $m_s = 0,\ -1\ m_I = 0,\ 1$ subspace, in order to calculate the optimal control pulse more conveniently, we reduced $H_0$ to a four level system

$$H_0 = A_{\parallel} S_z I_z - \frac{A_{\parallel}}{2} I_z, \tag{S8}$$

$$H_1 = \frac{\gamma_e u_1(t)}{\sqrt{2}} S_x, \tag{S9}$$

$$H_2 = \frac{\gamma_e u_2(t)}{\sqrt{2}} S_y, \tag{S10}$$

$$H_3 = \frac{\gamma_n u_3(t)}{\sqrt{2}} (\frac{\alpha_0 + \alpha_{-1}}{2} + (\alpha_0 - \alpha_{-1}) S_z) I_x, \tag{S11}$$

$$H_4 = \frac{\gamma_n u_4(t)}{\sqrt{2}} (\frac{\alpha_0 + \alpha_{-1}}{2} + (\alpha_0 - \alpha_{-1}) S_z) I_y. \tag{S12}$$

Where $u_i(t)$ is the amplitude varying with time. $\alpha_0$ and $\alpha_{-1}$ are the enhancement factors of the nuclear gyromagnetic ratio. They are

$$\alpha_0 = 1 - \frac{\gamma_e}{\gamma_n}\left(\frac{A_\perp}{D + \gamma_e B_z} + \frac{A_\perp}{D - \gamma_e B_z}\right), \tag{S13}$$

$$\alpha_{-1} = 1 + \frac{\gamma_e}{\gamma_n}\frac{A_\perp}{D - \gamma_e B_z}. \tag{S14}$$

### 1.2 Optimal Control Pulses

Due to the limitation of the short coherence time of NV center (1.7 $\mu s$), and imperfection of the control sequence, we used optimal control pulse to approximate the adiabatic evolution process. Here we adopted gradient ascent pulse engineering (GRAPE) algorithm [1]. We start form Eq. S8- S12, and take the spin bath noise and microwave amplitude fluctuation noise into consideration. Each sequence has 80 pieces, and the length is 196 $ns$ per piece.

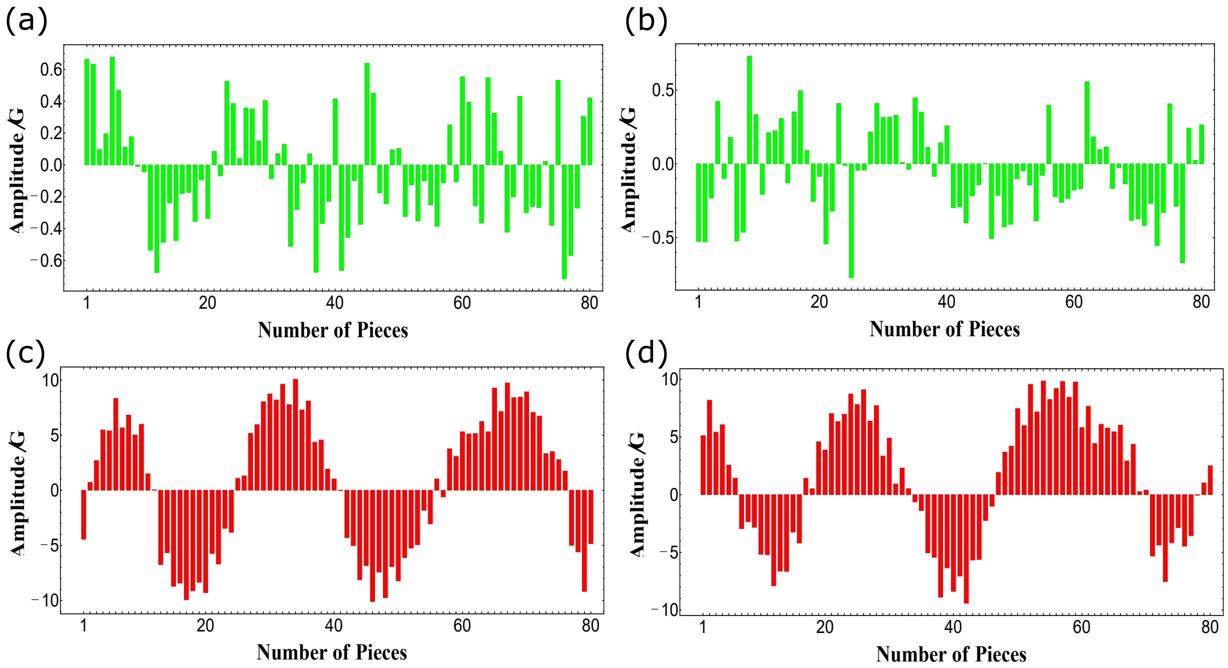


FIG. S1. RF and MW amplitude in the GRAPE pulse, the greens ones are the real and imaginary parts of MW sequence and the red ones are the real and imaginary parts of the RF sequence.

### 1.4 Simulations

By setting $s(t) = \frac{t}{T}$ in Eq.(1) in the main text we can get

$$H(t) = (1 - \frac{t}{T})g_2(S_x + I_x) + \frac{t}{T}g_1(2S_zI_z). \tag{S15}$$

As perfect adiabatic evolution only reaches when $T \to \infty$ , in practice we choose a finite time and do the simulations. If we choose $g1 = g2 = 2\pi\ MHz, T = 2\ \mu s$ and the initial state to be

$$|\psi_g(0)\rangle = (\frac{|0\rangle - |1\rangle}{\sqrt{2}})^{\otimes 2}. \tag{S16}$$

We can get the simulation results as shown in the left column of Fig. S2. In the continuous case, in the end the population on states $|00\rangle$, $|01\rangle$, $|10\rangle$ and $|11\rangle$ are 0.0062, 0.4938, 0.4938, 0.0062 respectively, the population concentrates on $|01\rangle$ and $|10\rangle$ states indicates that the solution is $\{p = 1,\ q = 0\}$ or $\{p = 0,\ q = 1\}$

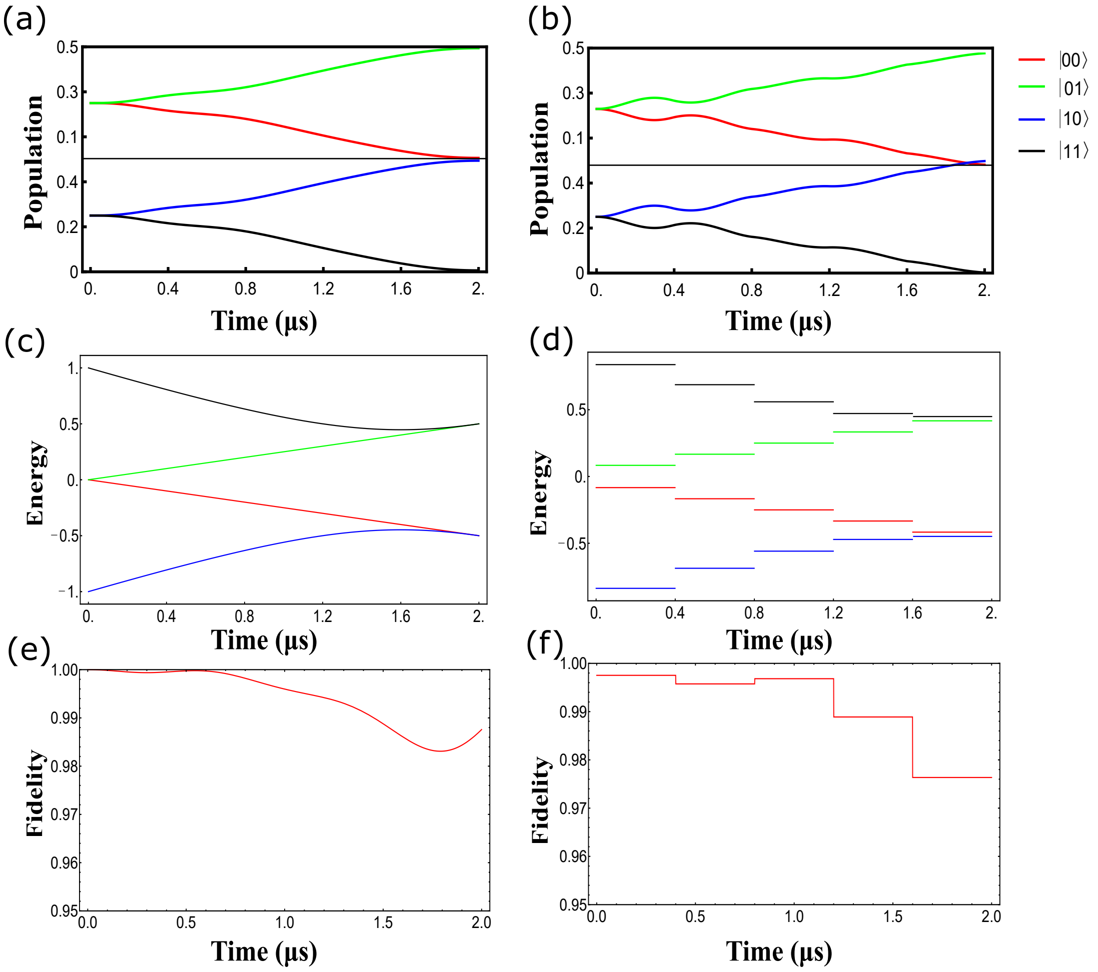


FIG. S2. The right column depicts the continuous adiabatic evolution process with $T = 2\ \mu s$. The left column shows the adiabatic evolution process discretized into 6 pieces. Each row, from top to the bottom, represents the population, energy and fidelity with the ground state during the evolution.

Since continuous variation of parameters is hard to achieve in real experiment, we discretize the Hamiltonian and sample it at certain times. The Hamiltonian after discretization is

$$H_\eta = 2\pi(1-\eta)(S_x + I_x) + 2\pi\eta(2S_zI_z), \tag{S17}$$

in which $\eta = \frac{i}{6}, i = 1, 2...5$, i.e., we divide the whole process into 6 pieces. From the right column of Fig. S2 we can see, after discretization the fidelity with the ground state is still good during the evolution, and at last the population on the computation basis is 0.0022, 0.4978, 0.4978 and 0.0022. which also gives the right answer of the problem.

### 1.5 Reduction of the classical equations

Form the multiplication table in the main text we get the equation set

$$p + q = 1 + 2z_{12}, \tag{S18}$$

$$1 + pq + 1 + z_{12} = 0 + 2z_{23} + 4z_{24}, \tag{S19}$$

$$p + q + z_{23} = 0 + 2z_{34} + 4z_{35}, \tag{S20}$$

$$1 + z_{34} + z_{24} = 0 + 2z_{45}, \tag{S21}$$

$$z_{45} + z_{35} = 1. \tag{S22}$$

In order to solve these equations using fewer qubits, we simplify further by utilizing the following logical constraints:

P1: if $x + y = 1$, then $xy = 0$;

P2: if $x + y + ... = az + b$ and $a > n - b$, n equals the number of variables on the left side, then $z = 0$;

P3: if $x + y + ... + 1 = az$, then $z = 1$;

and finally we get:

$$p + q = 1, \tag{S23}$$

this is exactly the Eq.(3) in the main text.

## EXPERIMENTAL METHODS

### 2.1 Confocal microscope and the sample

The experiments were carried out with our home-built confocal microscope. The sample used here is a chemical vapor deposition grown bulk diamond with [100] faces. The NV center is about 8 $\mu$m under the surface. A solid immersion lens was etched above the NV center to increase the counts. The $^{13}$C was at the natural abundance and the nitrogen impurity is less than 5 ppb.

### 2.2 Static field and microwave

The static magnetic field was supplied by a permanent magnet, it's 513 G along the NV axis. The MW and the RF pulses were generated by Agilent arbitrary wave generator M8190A, then passed two amplifiers working at different bands. The MW and RF then combined by a duplexer and transmitted to NV center though a coplanar waveguide (CPW). The MW and RF frequencies are 1436.4 MHz and 5.098 MHz respectively, corresponding to the transition from $|m_s = 0\rangle$ to $|m_s = -1\rangle$ and $|m_I = 0\rangle$ to $|m_I = 1\rangle$.

### 2.3 Experimental pulse sequences and data normalization

Generally the whole pulse sequence consists of three steps. First the green laser which lasts for 3 $\mu$s initialized the electron spin to $|m_s = 0\rangle$ state. Then the desired MW and RF pulse was applied. At last, to readout the electron spin state, the green laser was shinned again. Typically the whole sequence was repeated $10^6$ times to lower the shot noise. The initial state and final state after the evolution were characterized by quantum state tomography. Standard tomography flow can be found in [2]. Due to the different luminance of the levels, we added a normalization sequence at the end of every reading cycle. Assuming that a perfect initialization to state $|00\rangle$ is achieved at the

beginning. Denote $P_i$ as the population on level i, $L_i$ the luminance of the level, $S_i$ the counts after four different pulse sequence ($i = 1, 2, 3, 4$), the normalization sequence is as follows. Firstly readout without any pulse, the counts $S_1 = P_1 L_1$, secondly a RF pulse is applied and the counts $S_2 = P_1 L_2$, thirdly readout after a MW1 microwave pulse, and $S_3 = P_1 L_3$, at last RF and and MW2 are applied consecutively lead to $S_4 = P_1 L_4$. Perfect initialization means $P_1 = 1$, so we can get $L_i$ from the above equations.

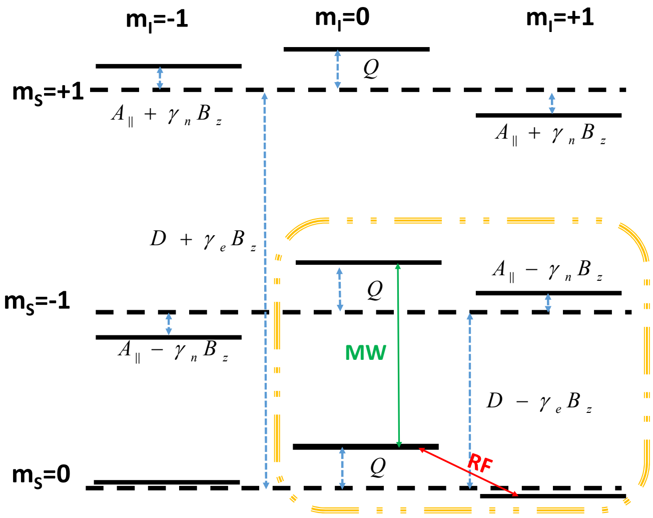


FIG. S3. **Energy levels of the NV-$^{14}$N coupling system.** There are totaly nine levels here, the experiment is carried out in the subspace spanned by $m_s = 0, m_s = -1$ and $m_I = 0, m_I = 1$ (in the orange box).

### 2.4 RF influence on MW

In the GRAPE pulse, there are sometime we applied RF and MW simultaneously. And there are two kinds of effects that RF may disturb the MW operations. One is the so called Bloch-Siegert Shift [3], which results in the energy level of $m_s = +1$ moving upward

$$\Delta\nu_{+1} = (\frac{\gamma_e B_{rfx}}{\sqrt{2}})^2 \frac{1}{2(D + \gamma_e B_{0z})}, \tag{S24}$$

$m_s = -1$ moving upward

$$\Delta\nu_{-1} = (\frac{\gamma_e B_{rfx}}{\sqrt{2}})^2 \frac{1}{2(D - \gamma_e B_{0z})}, \tag{S25}$$

$m_s = 0$ moving downward

$$\Delta\nu_{0} = (\frac{\gamma_e B_{rfx}}{\sqrt{2}})^2 (\frac{1}{2(D - \gamma_e B_{0z})} + \frac{1}{2(D + \gamma_e B_{0z})}), \tag{S26}$$

so the MW between $m_s = 0$ and $m_s = -1$ should have an extra detuning

$$\Delta\nu_{0\to-1} = (\frac{\gamma_e B_{rfx}}{\sqrt{2}})^2 (\frac{1}{(D - \gamma_e B_{0z})} + \frac{1}{2(D + \gamma_e B_{0z})}), \tag{S27}$$

and the MW between $ms = 0$ and $ms = +1$ should have an detuning

$$\Delta\nu_{0\to+1} = (\frac{\gamma_e B_{rfx}}{\sqrt{2}})^2(\frac{1}{(D+\gamma_e B_{0z})} + \frac{1}{2(D-\gamma_e B_{0z})}). \tag{S28}$$

Besides, the $x$ component (parallel to the NV axis) of the RF field serve to rotate the nuclear spin, however the z component (perpendicular to the NV axis) of the RF field has a disturbance on the electron spin energy level, as a result the MW frequency will mismatch the transition frequency (Fig. S4). In order to correct this RF influence, we need first measure $\frac{B_{rfz}}{B_{rf}}$, and then we also add an additional phase term in the MW sequence to cancel it.

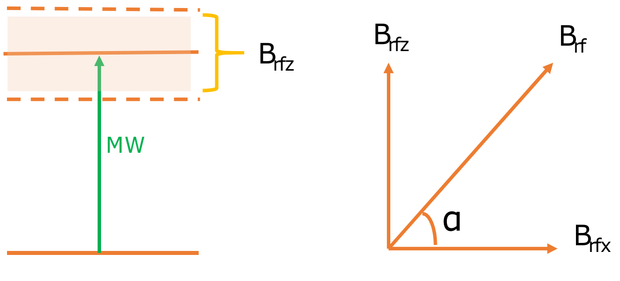


FIG. S4. **Illustration of the $B_{rf}$ direction and $B_{rfz}$ influence on mw**.

$B_{rfx}$ can be derived from the Rabi frequency of nuclear spin. $B_{rfz}$ can be measured in the following way. When carrying out standard Hahn echo sequence on electron spin, we insert a section of RF pulse between the first $\frac{\pi}{2}$ and $\pi$ pulse, the phase accumulated during the process is

$$\psi = 2\pi\frac{\gamma_e B_{rfz}}{\omega_{rf}}(Sin(2\pi\omega_r f + \psi_0) - Sin(\psi_0)), \tag{S29}$$

from which we can get $B_{rfz}$. The effect of the cancelation can be verified by using MW continuously driving the electron spin and apply the RF pulse at the same time. As Fig. S5 shows that the Rabi nutation of the electron spin with and without RF applied are nearly the same, which indicates that the cancelation method works pretty well.

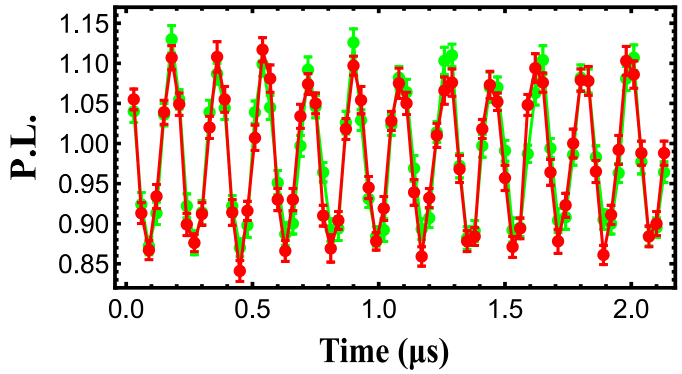


FIG. S5. **Cancelation effect**. Rabi nutation of the electron spin with (green dot) and without (red dot) RF applied are nearly the same.


[1] N. Khaneja, T. Reiss, C. Kehlet, T. Schulte-Herbrggen, and S. J. Glaser, J. Magn. Reson. **172**, 296 (2005).

[2] P. Neumann, N. Mizuochi, F. Rempp, P. Hemmer, H. Watanabe, S. Yamasaki, V. Jacques, T. Gaebel, F. Jelezko, and J. Wrachtrup, Science **320**, 1326 (2008).

[3] F. Bloch and A. Siegert, Phys. Rev. **57**, 522 (1940).
